# Supplementary material for: Unifying Identification and Context Learning for Person Recognition
Source: arXiv:1806.03084 source file (2018-06-08)
Supplement: Supplementary file 1 [file supplemental.tex]

\section{New Dataset: Cast In Movies}

We show more details about our dataset -- \emph{Cast In Movies (CIM)} in Tab.~\ref{tab:dataset_statistics} and more examples in Figure~\ref{fig:dateset}.

\begin{table}[!thb]
	\centering
	\vspace{-5pt}	
	\begin{tabular}{|c|c|c|c|c|}
		\hline
		& Train & Val   & Test  & Total  \\
		\hline
		Movies          & 115   & 19    & 58    & 192    \\
		Images          & 45,491 & 8,590  & 18,794 & 72,875  \\
		Cast Identities & 739   & 147   & 332   & 1,218   \\
		Instances       & 93,993 & 17,775 & 38,754 & 150,522 \\
		Avg/identity    & 67.54 & 58.78 & 57.35 & 63.70  \\
		Min/identity    & 5     & 5     & 10    & 5      \\
		Max/identity    & 1,177  & 355   & 610   & 1,177   \\
		\hline  
	\end{tabular}
	\caption{Statistics of CIM dataset}
	\label{tab:dataset_statistics}
\end{table}

\section{Region Detection}
As mentioned in our paper, we follow a certain procedure to get region locations. For ``head'' in \emph{PIPA}~\cite{zhang2015beyond} and ``body'' in \emph{CIM}, we simply use the annotations. For ``face'', we use a face detector~\cite{zhang2016joint} to get face bounding boxes and landmarks. Then we align ``face'' to a standard shape via translation, rotation, and scaling. For other regions, we use OpenPose~\cite{cao2016realtime} to get body landmarks
and also align them to a standard shape via translation, rotation, and scaling.
Figure~\ref{fig:align} shows the procedure of aligning and croping.
For example, for ``face'', we align it by the locations of ``eyes'' and ``nose'' and crop it with a $255 \times 255$ rectangle.

\begin{figure}[h]
	\centering
	\includegraphics[width=\linewidth]{align}
	\caption{\small
		Procedure of aligning and croping
	}
	\label{fig:align}
\end{figure}

Notice that we only keep those bounding boxes that lie mostly within the photo.
For example, for ``face'', we only keep the instances whose ``eyes'' and ``nose'' are detected.
For those regions that are largely invisible, we simply use a black image to represent their appearance. 
Tab.~\ref{tab:visible} show the percentage of visible samples of different regions in \emph{PIPA} and \emph{CIM}.
As ``head'' in \emph{PIPA} and ``body'' in \emph{CIM} come from annotation,
so they are 100\% visible.
From the percentage of the samples whose ``face'' are visible in \emph{PIPA} and \emph{CIM} (69.96\% vs. 53.06\%), we can also see that \emph{CIM} is more challenging.

\begin{table}[]
	\centering
	\begin{tabular}{|c|cccc|}
		\hline
		& head    & face    & upperbody & body    \\ \hline
		PIPA & 100\%   & 69.96\% & 84.86\%   & 82.19\% \\ \hline
		CIM  & 70.70\% & 53.06\% & 98.99\%   & 100\%   \\ \hline
	\end{tabular}
	\caption{Percentage of visible samples of different regions.}
	\label{tab:visible}
\end{table}

\section{Compared with Single Region Models}

Tab.~\ref{tab:perform_single} shows the performances of single region models.
For example, ``head'' means we only use the feature of ``head'' region for matching. We can see the effectiveness of visual cues combination by comparing the performances with single region models.

\begin{table*}[!h]
	\centering
	\begin{tabular}{|c|c|cccc|cc|}
		\hline
		\multicolumn{2}{|l|}{}           & head    & face    & upperbody & body    & RANet fusion & full model       \\ \hline
		\multirow{4}{*}{PIPA} & origianl & 81.63\% & 63.81\% & 61.56\%   & 61.15\% & 87.33\%      & \textbf{89.73\%} \\ \cline{2-8} 
		& album    & 73.63\% & 62.52\% & 53.88\%   & 53.10\% & 82.59\%      & \textbf{85.33\%} \\ \cline{2-8} 
		& time     & 64.77\% & 60.77\% & 44.70\%   & 43.87\% & 76.52\%      & \textbf{80.42\%} \\ \cline{2-8} 
		& day      & 46.01\% & 60.27\% & 22.42\%   & 19.48\% & 65.49\%      & \textbf{67.16\%} \\ \hline
		\multicolumn{2}{|c|}{CIM}        & 50.30\% & 53.09\% & 55.35\%   & 55.02\% & 71.93\%      & \textbf{74.40\%} \\ \hline
	\end{tabular}
	\caption{Performance compared with single region models.}
	\label{tab:perform_single}
\end{table*}

\section{Case Visulization}

Figure~\ref{fig:event_pipa} and Figure~\ref{fig:event_cim} show more examples of ``events'' automatically discovered by our approach respectively from \emph{PIPA} and \emph{CIM}.
Images in each row belong to the same ``event''.

Figure~\ref{fig:case0}, \ref{fig:case1}, \ref{fig:case2}, \ref{fig:case3} show more examples of recognition results from \emph{PIPA} and \emph{CIM}.
For each photo, the mark at the top left corner indicates whether the corresponding method predicts correctly for the highlighted instance.
We can see that ``face recognition'' can only handle the instances with frontal and clear faces (Figure~\ref{fig:case0}).
While ''RANet Fusion'', which combines different visual cues with instance-dependent weights, can still correctly recognize persons when ``face'' is not clearly visible (Figure~\ref{fig:case1}).
For more challenging cases, our full model can still make a correct prediction by exploiting the social context (Figure~\ref{fig:case2}).
But there are also some very difficult cases where all the methods fail (Figure~\ref{fig:case3}).

\begin{figure*}[h]
	\centering
	\includegraphics[width=\linewidth]{dateset_a_lot}
%	\vspace{-10pt}
	\caption{
		Examples from our proposed dataset -- \emph{Cast In Movies (CIM)}.
	}
	\label{fig:dateset}
	\vspace{-10pt}
\end{figure*}

\begin{figure*}[thb]
\centering
\includegraphics[width=\linewidth]{event_pipa}
\vspace{-10pt}
\caption{
	Examples of ``events'' in \emph{PIPA}.
}
\label{fig:event_pipa}
\vspace{-10pt}
\end{figure*}

\begin{figure*}[thb]
	\centering
	\includegraphics[width=\linewidth]{event_cim}
	\vspace{-10pt}
	\caption{\small
		Examples of ``events'' in \emph{CIM}.
	}
	\label{fig:event_cim}
	\vspace{-10pt}
\end{figure*}

\begin{figure*}[thb]
	\centering
	\includegraphics[width=0.85\linewidth]{case0}
	\caption{
		Example photos and recognition results (a).
	}
	\label{fig:case0}
	\vspace{-10pt}
\end{figure*}

\begin{figure*}[thb]
	\centering
	\includegraphics[width=0.85\linewidth]{case1}
	\caption{
		Example photos and recognition results (b).
	}
	\label{fig:case1}
	\vspace{-10pt}
\end{figure*}

\begin{figure*}[thb]
	\centering
	\includegraphics[width=0.85\linewidth]{case2}
	\caption{
		Example photos and recognition results (c).
	}
	\label{fig:case2}
	\vspace{-10pt}
\end{figure*}

\begin{figure*}[thb]
	\centering
	\includegraphics[width=0.85\linewidth]{case3}
	\caption{
		Example photos and recognition results (d).
	}
	\label{fig:case3}
	\vspace{-10pt}
\end{figure*}
